# Supplementary material for: Generating Predicate Callback Summaries for the Android Framework
Source: arXiv:1703.08902 source file (2017-03-29)
Supplement: Supplementary file 1 [file appendix.tex]

\appendix 

We studied the use of 7 frequently invoked Android API calls in 546 F-Droid apps. In table \ref{tab:contextasc}, under {\it API}, we list 7 frequently invoked Android APIs, {\tt startService}, {\tt stopService}, {\tt bindService}, {\tt unbindService}, {\tt stopService} from the Service component, {\tt startActivity} and {\tt finish} from the Activity component. Under {\it Context}, we list which state the APIs has been invoked in the app (we use the name of the state given in the Android lifecycles). Under {\it No. Apps}, we report the number of apps that have placed the call listed in the first column in state listed in the second column. 
 
 \begin{table}[h]
 	\centering
 	\caption{APIs Invoked in Different Contexts\label{tab:contextasc}}
 	\begin{tabular}{l|l|c}
 		\hline
 		AFC & Context & No. Apps \\ \hline\hline
 		%\multicolumn{3}{|c|}{Service} \\ \hline   
 		\multirow{4}{*}{startService} & Initial & 99 \\
 		& Started & 20  \\
 		& Bound & 11  \\
 		& StartedBound & 5  \\ \hline
 		\multirow{2}{*}{stopService} & Started & 35  \\
 		& StartedBound & 5 \\ \hline
 		\multirow{3}{*}{bindService} & Initial & 28  \\
 		& Started & 15  \\
 		& StartedBound & 3  \\ \hline
 		\multirow{2}{*}{unbindService} & Bound & 25 \\
 		& StartedBound & 14 \\ \hline
 		\multirow{4}{*}{stopSelf} & Initial & 8  \\
 		& Created & 35  \\
 		& Started & 4  \\
 		& StartedBound & 15 \\ \hline\hline
 		%\multicolumn{3}{|c|}{Activity} \\ \hline
 		\multirow{3}{*}{startActivity} & Initial & 281  \\
 		& Active & 25  \\
 		& Paused & 20  \\ \hline
 		\multirow{4}{*}{finish} & Initial & 177  \\
 		& Active & 315  \\
 		& Paused & 8  \\
 		& Stopped & 10 \\ \hline
 	\end{tabular}
 \end{table}
